# Supplementary material for: Demystifying Spatial Confounding
Source: arXiv:2309.16861 source file (2025-07-14)
Supplement: Supplementary file 1 [file appendix.pdf]

# Supporting Information for “Demystifying Spatial Confounding” by E. Dupont, I. Marques and T. Kneib

July 1, 2025

**Abstract**

In this appendix, we provide proofs as well as additional analysis and simulation results, supporting the material in the main paper.

# 1 Proofs and theoretical results

## 1.1 The spatial precision matrix $\Sigma^{-1}$

Central to our analyses are the properties of the precision matrix $\Sigma^{-1}$, in particular, its eigenvalues, which are computed in Lemma 1. First we have the following preliminary results.

**Lemma A.1.** *The inverse of the covariance structure $\Sigma$ is given by $\Sigma^{-1} = \sigma^{-2}(\mathbf{I} - \mathbf{A})$, where $\mathbf{A} = \sigma^{-2}\mathbf{B}_{\text{sp}}(\sigma^{-2}\mathbf{B}_{\text{sp}}^T\mathbf{B}_{\text{sp}} + \lambda\mathbf{S})^{-1}\mathbf{B}_{\text{sp}}^T$ is the influence matrix of a purely spatial model, i.e. a model only containing the spatial effect.*

*Proof.* Let $\mathbf{M} = \sigma^{-2}(\mathbf{I} - \mathbf{A})$. Then

$$\begin{aligned}
\Sigma\mathbf{M} &= (\sigma^2\mathbf{I} + \lambda^{-1}\mathbf{B}_{\text{sp}}\mathbf{S}^-\mathbf{B}_{\text{sp}}^T)\left(\sigma^{-2}\mathbf{I} - \sigma^{-4}\mathbf{B}_{\text{sp}}(\sigma^{-2}\mathbf{B}_{\text{sp}}^T\mathbf{B}_{\text{sp}} + \lambda\mathbf{S})^{-1}\mathbf{B}_{\text{sp}}^T\right) \\
&= \mathbf{I} + \sigma^{-2}\lambda^{-1}\mathbf{B}_{\text{sp}}\mathbf{S}^-\mathbf{B}_{\text{sp}}^T - \sigma^{-2}\mathbf{B}_{\text{sp}}(\sigma^{-2}\mathbf{B}_{\text{sp}}^T\mathbf{B}_{\text{sp}} + \lambda\mathbf{S})^{-1}\mathbf{B}_{\text{sp}}^T \\
&\quad -\sigma^{-4}\lambda^{-1}\mathbf{B}_{\text{sp}}\mathbf{S}^-\mathbf{B}_{\text{sp}}^T\mathbf{B}_{\text{sp}}(\sigma^{-2}\mathbf{B}_{\text{sp}}^T\mathbf{B}_{\text{sp}} + \lambda\mathbf{S})^{-1}\mathbf{B}_{\text{sp}}^T \\
&= \mathbf{I} + \sigma^{-2}\lambda^{-1}\mathbf{B}_{\text{sp}}\mathbf{S}^-\left(\mathbf{I} - (\lambda\mathbf{S} + \sigma^{-2}\mathbf{B}_{\text{sp}}^T\mathbf{B}_{\text{sp}})(\sigma^{-2}\mathbf{B}_{\text{sp}}^T\mathbf{B}_{\text{sp}} + \lambda\mathbf{S})^{-1}\right)\mathbf{B}_{\text{sp}}^T \\
&= \mathbf{I}.
\end{aligned}$$

Hence $\Sigma^{-1} = \mathbf{M}$.

□

**Lemma A.2.** *Let $\alpha_1 \leq \cdots \leq \alpha_p$ be the eigenvalues of the penalty matrix $\mathbf{S}$ and $\lambda > 0$ the smoothing parameter. Then the influence matrix $\mathbf{A} = \sigma^{-2}\mathbf{B}_{\text{sp}}(\sigma^{-2}\mathbf{B}_{\text{sp}}^T\mathbf{B}_{\text{sp}} + \lambda\mathbf{S})^{-1}\mathbf{B}_{\text{sp}}^T$ is symmetric positive semi-definite and its eigenvalues are given by $\{0, \alpha_1', \ldots, \alpha_p'\}$ where $\alpha_i' = \sigma^{-2}/(\sigma^{-2} + \lambda\alpha_i)$ for $i = 1, \ldots, p$.*

*Proof.* As $\mathbf{S}$ is symmetric, $\mathbf{A}$ is also symmetric. Without loss of generality we can assume that the spatial basis $\mathbf{B}_{\text{sp}}$ is orthonormal so that $\mathbf{B}_{\text{sp}}^T\mathbf{B}_{\text{sp}} = \mathbf{I}$ and

$$\mathbf{A} = \sigma^{-2}\mathbf{B}_{\text{sp}}(\sigma^{-2}\mathbf{I} + \lambda\mathbf{S})^{-1}\mathbf{B}_{\text{sp}}^T.$$

Clearly anything in the null space of $\mathbf{A}$ (i.e. the orthogonal complement of the column space of $\mathbf{B}_{\text{sp}}$, which is the "non-spatial" part of $\mathbb{R}^n$) is an eigenvector with eigenvalue 0.

Suppose $\mathbf{v} \in \mathbb{R}^p$ is an eigenvector of $\mathbf{S}$ with eigenvalue $\alpha_i$. Let $\mathbf{v}' = \mathbf{B}_{\text{sp}}\mathbf{v}$. Then $\mathbf{v}' \in \mathbb{R}^n$ and

$$\begin{aligned}
\mathbf{A}\mathbf{v}' &= \sigma^{-2}\mathbf{B}_{\text{sp}}(\sigma^{-2}\mathbf{I} + \lambda\mathbf{S})^{-1}\mathbf{B}_{\text{sp}}^T\mathbf{B}_{\text{sp}}\mathbf{v} \\
&= \sigma^{-2}\mathbf{B}_{\text{sp}}(\sigma^{-2}\mathbf{I} + \lambda\mathbf{S})^{-1}\mathbf{v} \\
&= \sigma^{-2}\mathbf{B}_{\text{sp}}(\sigma^{-2} + \lambda\alpha_i)^{-1}\mathbf{v} \\
&= \tfrac{\sigma^{-2}}{\sigma^{-2}+\lambda\alpha_i}\mathbf{v}'.
\end{aligned}$$

Since all eigenvalues are non-negative, $\mathbf{A}$ is positive semi-definite. □

Lemma A.2 gives some insight into the mechanism of smoothing within the spatial data analysis model (3). Since $\mathbf{A}$ is the influence matrix of a purely spatial model, the estimated spatial effect in model (3) is given by $\widehat{\mathbf{z}} = \mathbf{B}_{\text{sp}}\widehat{\beta}_{\text{sp}} = \mathbf{A}(\mathbf{y} - \widehat{\beta}\mathbf{x})$. So each eigenvalue of $\mathbf{A}$ tells us how much weight the corresponding eigenvector is given within the estimated spatial effect. The "non-spatial" part of $\mathbb{R}^n$ is spanned by eigenvectors with eigenvalue 0 and therefore contributes nothing to the estimated spatial effect. The remaining eigenvalues $\alpha'_1, \ldots, \alpha'_p$ satisfy $0 < \alpha'_p \leq \cdots \leq \alpha'_1 \leq 1$ with $\alpha'_i = 1$ if and only if $\lambda\alpha_i = 0$. Since $\lambda > 0$, only unpenalised spatial basis vectors (i.e. eigenvectors with $\alpha_i = 0$) are given the maximum weight of 1 in the estimated spatial effect. For all other spatial basis vectors, smoothing reduces the weight of the contribution to less than 1, and the larger the value of $\alpha_i$ (i.e. the higher the penalisation) the smaller the contribution of the corresponding eigenvector. As higher frequency eigenvectors are typically those with the highest penalisation, these contribute least to the estimated spatial effect in line with intuition.

The smoothing parameter $\lambda$ controls the overall level of smoothing with larger values of $\lambda$ (i.e. more smoothing) leading to a smaller contribution of all spatial basis vectors to the estimated effect. At the other extreme ($\lambda \to 0$) is an entirely unsmoothed spatial effect which gives the maximum weight of 1 to all eigenvectors.

Combining Lemmas A.1 and A.2 we can now prove Lemma 1:

*Proof of Lemma 1.* By Lemma A.1 we have that $\Sigma^{-1} = \sigma^{-2}(\mathbf{I} - \mathbf{A})$ so the eigenvalues of $\Sigma^{-1}$ are all of the form $\sigma^{-2}(1 - \alpha)$ where $\alpha$ is an eigenvalue of $\mathbf{A}$. Lemma A.2 gives us the eigenvalues of $\mathbf{A}$. The eigenvalue $\alpha = 0$ (corresponding to the eigenvectors spanning the non-spatial part of $\mathbb{R}^n$) leads to the eigenvalue $\sigma^{-2}$ for $\Sigma^{-1}$ and the remaining eigenvalues of $\Sigma^{-1}$ are given by

$$\sigma^{-2}(1 - \tfrac{\sigma^{-2}}{\sigma^{-2}+\lambda\alpha_i}) = \tfrac{\sigma^{-2}\lambda\alpha_i}{\sigma^{-2}+\lambda\alpha_i}, \quad \text{for } i = 1, \ldots, p.$$

□

## 1.2 Spatial frequencies

Although the spatial confounding literature often emphasises the importance of spatial frequencies, there is no single definition of what spatial frequencies are. In the seminal work of Paciorek (2010), and later Page et al. (2017), who considered the impact of spatial scales on spatial confounding in Gaussian process models, spatial scale was defined through the model parameters. More recent work such as Guan et al. (2023) and Keller and Szpiro (2020) use spectral frequencies, i.e. spatial Fourier expansions. Keller and Szpiro (2020) also suggest analysing spatial behaviour using wavelets. While Fourier and wavelet analyses are well-established exploratory tools for investigating frequency behaviours, they have some disadvantages, e.g. Fourier analysis assumes spatial stationarity (which may be unrealistic in practice), and wavelet analysis requires subjective choices around the type of wavelet basis, the smoothness of basis functions etc. For discrete spatial models the notion of spatial frequencies is perhaps even harder to define, but e.g. for the ICAR random effects model with one data point per region, Guan et al. (2023) use eigenvectors related to the spatial precision matrix of the model.

In this paper, irrespective of whether the spatial analysis model is discrete or continuous and the choice of the spatial effect, we use the eigenvectors of the precision matrix $\mathbf{\Sigma}^{-1}$ to represent different spatial frequencies. Here we show in more detail how these eigenvectors form a natural representation of spatial frequencies. Firstly, for all spatial models, the underlying assumption is that nearby observations are more similar than observations far apart. Therefore, irrespective of the exact specification of the spatial random effect, the resulting smoothing penalty $\mathbf{S}$ is designed to penalise abrupt local changes (interpretable as high frequency spatial behaviour) more than changes that occur over larger distances (interpretable as low frequency behaviour). In other words, the penalty structure encodes, in a quantifiable way, what the model perceives as high versus low frequency spatial behaviour.

For a given choice of spatial analysis model, we now consider the $n$ eigenvectors of the precision matrix $\mathbf{\Sigma}^{-1}$. Each eigenvector represents a particular behaviour over space, and Lemma 1 shows that the size of the corresponding eigenvalue is directly linked to how much that behaviour is penalised. More specifically, there are $n - p$ eigenvectors with eigenvalue $\sigma^{-2}$, i.e. these behaviours are unaffected by penalisation and can therefore be considered to be "non-spatial", and for the remaining $p$ eigenvectors, the eigenvalues are given by

$$\sigma^{-2} w_i, \quad w_i = \lambda \alpha_i / (\sigma^{-2} + \lambda \alpha_i)$$

with $\alpha_1 \leq \cdots \leq \alpha_p$ the eigenvalues of the penalty matrix $\mathbf{S}$. Although these $p$ eigenvalues depend on the parameters $\sigma^{-2}$ and $\lambda$ (which are usually estimated), their ordering is the same as the $\alpha_i$'s, i.e. $\sigma^{-2} w_1 \leq \cdots \leq \sigma^{-2} w_p$. Thus, irrespective of the estimates of the parameters, a large/small eigenvalue corresponds exactly to high/low penalisation. Therefore, if we order the $p$ spatial eigenvectors in ascending order of eigenvalues, the lowest spatial frequencies will be first and the highest spatial frequencies last. We illustrate this here using two examples (one discrete and one continuous).

### Example 1: Slovenia municipalities (discrete space model)

In this example we consider an ICAR random effects model with one observation in each region using the $n = 212$ municipalities of Slovenia. In this case, the spatial random effect has dimension $p = n$ so we can use the orthonormal spatial basis $\mathbf{B}_{\text{sp}} = \mathbf{I}$ (as the spatial basis simply spans the whole space). The penalty matrix $\mathbf{S}$ is the graph Laplacian of the neighbourhood structure defined by the map in Figure 1 (left). The spatial precision matrix is given by $\mathbf{\Sigma}^{-1} = \sigma^{-2}(\mathbf{I} - \mathbf{A})$ where $\mathbf{A} = \sigma^{-2}(\sigma^{-2}\mathbf{I} + \lambda\mathbf{S})^{-1}$. The $n$ eigenvectors of $\mathbf{\Sigma}^{-1}$ are therefore equal to the $p = n$ eigenvectors of $\mathbf{S}$ and there are no non-spatial eigenvectors.

The eigenvalues $\alpha_1 \leq \cdots \leq \alpha_n$ of $\mathbf{S}$ in ascending order are shown in Figure 1 (right). The eigenvalues of $\mathbf{\Sigma}^{-1}$ are given by $\sigma^{-2}w_1 \leq \cdots \leq \sigma^{-2}w_n$ where $w_i = \lambda\alpha_i/(\sigma^{-2} + \lambda\alpha_i)$. Figure 2 shows plots of four different eigenvectors in ascending order of eigenvalues. As expected, low/high eigenvalues result in low/high spatial frequency behaviours.

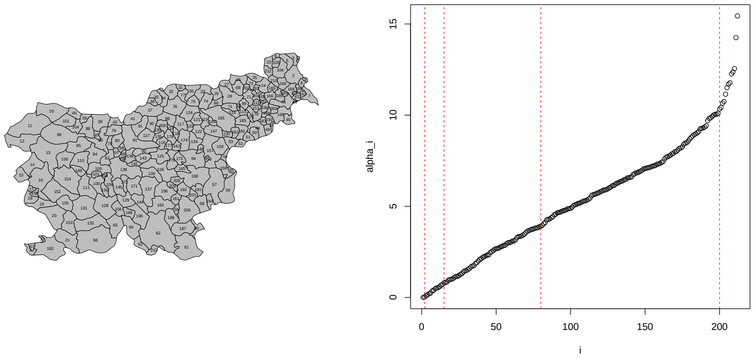


Figure 1: Slovenia example: Municipalities (left) and eigenvalues of $\mathbf{S}$ in ascending order with vertical red lines showing the four ($i = 2, 15, 80, 200$) used for the plots in Figure 2 (right).

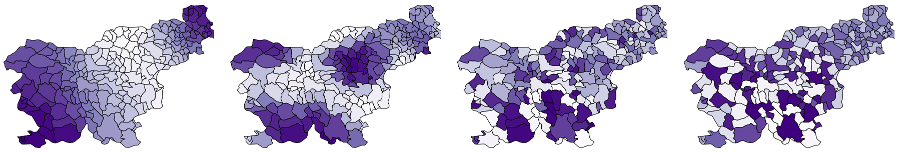

Figure 2: Slovenia example: Four spatial eigenvectors ($i = 2, 15, 80, 200$) of $\mathbf{\Sigma}^{-1}$ in ascending order of eigenvalues from left to right.

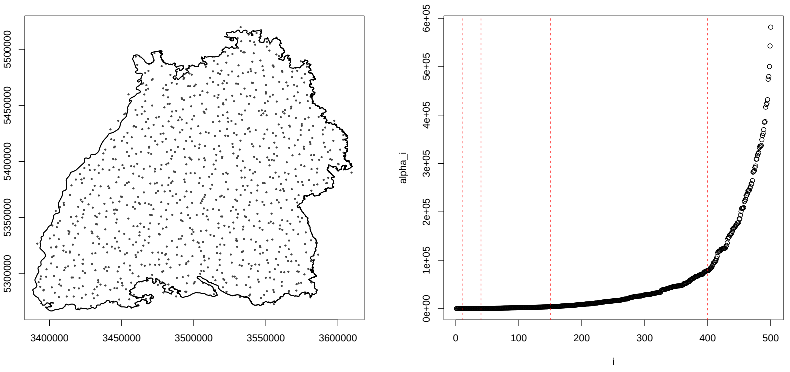


Figure 3: Baden-Württemberg example: Data locations (left) and eigenvalues of $\mathbf{S}$ in ascending order with vertical red lines showing the four ($i = 10, 40, 150, 400$) used for the plots in Figure 4

**Example 2: Baden-Württemberg (continuous space model)**

In this example we have sampled $n = 1000$ random locations across Baden-Württemberg, Germany (shown in Figure 3 (left)). We consider a thin plate regression spline model with $k = 500$ basis functions for the spatial effect. So $p = k < n$ and the model matrix for the spatial effect is the $n \times k$ matrix where each column is a thin plate spline basis function evaluated at the data locations (including a constant column of 1's that represents the intercept). We define $\mathbf{B}_{\text{sp}}$ to be the orthogonalised version of this model matrix (using Gram-Schmidt orthogonalisation). The matrix $\mathbf{S}$ is the $k \times k$ thin plate spline smoothing penalty (where the intercept has penalty 0) and the spatial precision matrix is the $n \times n$ matrix given by $\mathbf{\Sigma}^{-1} = \sigma^{-2}(\mathbf{I} - \mathbf{A})$ where $\mathbf{A} = \sigma^{-2}\mathbf{B}_{\text{sp}}(\sigma^{-2}\mathbf{I} + \lambda\mathbf{S})^{-1}\mathbf{B}_{\text{sp}}^T$.

The proof of Lemma A.1 shows that if $\mathbf{v}_1, \ldots, \mathbf{v}_k$ are the ($k$-dimensional) eigenvectors of $\mathbf{S}$ with eigenvalues $\alpha_1 \leq \cdots \leq \alpha_k$, then $\mathbf{v}'_i = \mathbf{B}_{\text{sp}}\mathbf{v}_i$, $i = 1, \ldots, k$, are the ($n$-dimensional) spatial eigenvectors of $\mathbf{\Sigma}^{-1}$ with eigenvalues $\sigma^{-2}w_1 \leq \cdots \leq \sigma^{-2}w_k$, $w_i = \lambda\alpha_i/(\sigma^{-2} + \lambda\alpha_i)$. The remaining $n - k$ eigenvectors of $\mathbf{\Sigma}^{-1}$ have eigenvalue $\sigma^{-2}$ and span the "non-spatial" part of the sample space. So we see that the eigendecomposition of $\mathbf{\Sigma}^{-1}$ somehow "translates" the smoothing that is specified in the smaller $k$-dimensional space into the $n$-dimensional sample space and gives a natural decomposition of the sample space into different spatial behaviours.

Figure 3 (right) shows the eigenvalues of $\mathbf{S}$ in ascending order. Figure 4 shows plots of four different spatial eigenvectors in ascending order of eigenvalues. As the eigenvectors are only defined at the data locations, we have also shown spatially interpolated versions of these (using thin plate regression splines with basis size 900 for the interpolations). Once again, the plots confirm that low/high eigenvalues result in low/high spatial frequency behaviours.

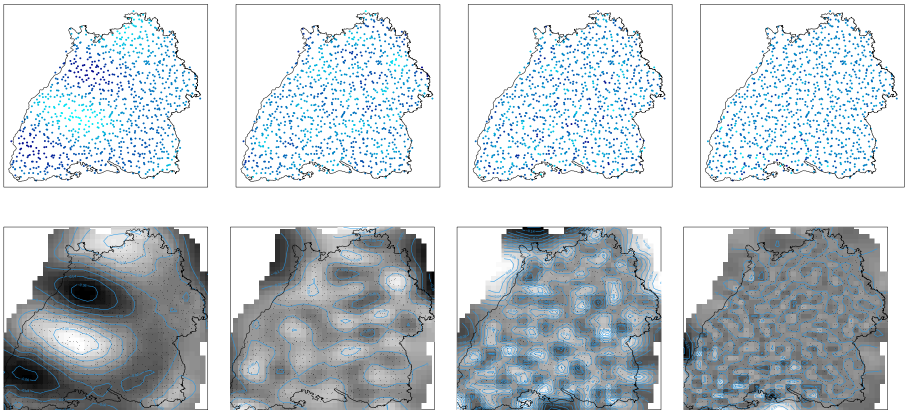

Figure 4: Baden-Württemberg example: Four eigenvectors ($i = 10, 40, 150, 400$) of $\mathbf{\Sigma}^{-1}$ in ascending order of eigenvalues from left to right (top). Smooth interpolations of the same four eigenvectors (bottom).

## 1.3 Proof of Proposition 1

*Proof.* Since under the data generating model (2) $\mathrm{E}(\mathbf{y}) = \beta\mathbf{x} + \mathbf{z}$, we have that

$$\begin{aligned}
\mathrm{E}(\widehat{\beta}) &= (\mathbf{x}^T\Sigma^{-1}\mathbf{x})^{-1}\mathbf{x}^T\Sigma^{-1}\,\mathrm{E}(\mathbf{y}) \\
&= (\mathbf{x}^T\Sigma^{-1}\mathbf{x})^{-1}\mathbf{x}^T\Sigma^{-1}(\beta\mathbf{x} + \mathbf{z}) \\
&= \beta + (\mathbf{x}^T\Sigma^{-1}\mathbf{x})^{-1}\mathbf{x}^T\Sigma^{-1}\mathbf{z} \\
&= \beta + \frac{\langle \mathbf{x}, \mathbf{z}\rangle_{\Sigma^{-1}}}{\langle \mathbf{x}, \mathbf{x}\rangle_{\Sigma^{-1}}}.
\end{aligned}$$

□

## 1.4 Proof of Corollary 1

*Proof.* The numerator of the bias in $\widehat{\beta}$ is given by

$$\begin{aligned}
\langle \mathbf{x}, \mathbf{z} \rangle_{\Sigma^{-1}} &= \mathbf{x}^T \Sigma^{-1} \mathbf{z} \\
&= \boldsymbol{\xi}^{xT} \mathbf{U}^T \Sigma^{-1} \mathbf{U} \boldsymbol{\xi}^z \\
&= \sigma^{-2} \boldsymbol{\xi}_{\text{ns}}^{xT} \boldsymbol{\xi}_{\text{ns}}^z + \sigma^{-2} \boldsymbol{\xi}_{\text{sp}}^{xT} \begin{bmatrix} w_1 & & \\ & \ddots & \\ & & w_p \end{bmatrix} \boldsymbol{\xi}_{\text{sp}}^z \\
&= \sigma^{-2} \boldsymbol{\xi}_{\text{sp}}^{xT} \begin{bmatrix} w_1 & & \\ & \ddots & \\ & & w_p \end{bmatrix} \boldsymbol{\xi}_{\text{sp}}^z \\
&= \sigma^{-2} \sum_{i=1}^{p} \xi_{\text{sp},i}^x \xi_{\text{sp},i}^z w_i.
\end{aligned}$$

Similarly, the denominator of the bias is given by

$$\begin{aligned}
\langle \mathbf{x}, \mathbf{x} \rangle_{\Sigma^{-1}} &= \sigma^{-2} \boldsymbol{\xi}_{\text{ns}}^{xT} \boldsymbol{\xi}_{\text{ns}}^x + \sigma^{-2} \boldsymbol{\xi}_{\text{sp}}^{xT} \begin{bmatrix} w_1 & & \\ & \ddots & \\ & & w_p \end{bmatrix} \boldsymbol{\xi}_{\text{sp}}^x \\
&= \sigma^{-2} \sum_{i=1}^{n-p} (\xi_{\text{ns},i}^x)^2 + \sigma^{-2} \sum_{i=1}^{p} (\xi_{\text{sp},i}^x)^2 w_i.
\end{aligned}$$

□

## 1.5 Comparison to the non-spatial model

Using the expressions in Corollaries 1 and 2, we compute the difference between the bias $\text{Bias}_{\text{ns}} = \text{E}(\widehat{\beta}_{\text{ns}}) - \beta$ in the non-spatial model (4) and the bias $\text{Bias} = \text{E}(\widehat{\beta}) - \beta$ in the spatial model (3). As we are mainly interested in comparing the size of the bias, for simplicity assume that all $\xi_{\text{sp},i}^x \xi_{\text{sp},i}^z$ are positive. To simplify notation, let

$$C_{\text{ns}} = \sum_{i=1}^{n-p} (\xi_{\text{ns},i}^x)^2 \geq 0.$$

Then,

$$\begin{aligned}
\text{Bias}_{\text{ns}} - \text{Bias} &= \frac{\sum_{i=1}^p \xi_{\text{sp},i}^x \xi_{\text{sp},i}^z}{C_{\text{ns}} + \sum_{i=1}^p (\xi_{\text{sp},i}^x)^2} - \frac{\sum_{i=1}^p \xi_{\text{sp},i}^x \xi_{\text{sp},i}^z w_i}{C_{\text{ns}} + \sum_{i=1}^p (\xi_{\text{sp},i}^x)^2 w_i} \\
&= \frac{\left(\sum_{i=1}^p \xi_{\text{sp},i}^x \xi_{\text{sp},i}^z\right) \left(C_{\text{ns}} + \sum_{i=1}^p (\xi_{\text{sp},i}^x)^2 w_i\right)}{\left(C_{\text{ns}} + \sum_{i=1}^p (\xi_{\text{sp},i}^x)^2\right) \left(C_{\text{ns}} + \sum_{i=1}^p (\xi_{\text{sp},i}^x)^2 w_i\right)} \\
&\quad - \frac{\left(\sum_{i=1}^p \xi_{\text{sp},i}^x \xi_{\text{sp},i}^z w_i\right) \left(C_{\text{ns}} + \sum_{i=1}^p (\xi_{\text{sp},i}^x)^2\right)}{\left(C_{\text{ns}} + \sum_{i=1}^p (\xi_{\text{sp},i}^x)^2\right) \left(C_{\text{ns}} + \sum_{i=1}^p (\xi_{\text{sp},i}^x)^2 w_i\right)}.
\end{aligned}$$

The denominator of this expression is positive and the numerator can be written as

$$C_{\text{ns}} \sum_{i=1}^{p} \xi^x_{\text{sp},i} \xi^z_{\text{sp},i} (1 - w_i) + \sum_{i,j} \xi^x_{\text{sp},i} \xi^z_{\text{sp},i} (\xi^x_{\text{sp},j})^2 (w_j - w_i).$$

Recall that $0 \leq w_1 \leq \cdots \leq w_p < 1$ and note that $\xi^x_{\text{sp},i}\xi^z_{\text{sp},i}$ is non-zero exactly when frequency $i$ is confounded. Therefore, the first term in the numerator is strictly positive whenever there is confounding and $\mathbf{x}$ has non-spatial information, and is larger when confounded frequencies in $\mathbf{x}$ have low weights (i.e. are the low frequencies). The second term can be written as

$$\sum_{i<j} (\xi^x_{\text{sp},i} \xi^z_{\text{sp},i} (\xi^x_{\text{sp},j})^2 - \xi^x_{\text{sp},j} \xi^z_{\text{sp},j} (\xi^x_{\text{sp},i})^2)(w_j - w_i).$$

Since $w_j - w_i \geq 0$ for $i < j$, this shows that confounding at low frequencies ($\xi^x_{\text{sp},i}\xi^z_{\text{sp},i} \neq 0$) contribute positively to the sum, whereas confounding at high frequencies ($\xi^x_{\text{sp},j}\xi^z_{\text{sp},j} \neq 0$) contribute negatively. Conversely, unconfounded high frequencies ($\xi^x_{\text{sp},j} \neq 0$, $\xi^z_{\text{sp},j} = 0$) contribute positively, while unconfounded low frequencies ($\xi^x_{\text{sp},i} \neq 0$, $\xi^z_{\text{sp},i} = 0$) contribute negatively. Note that for a fixed unconfounded high frequency $j$ the contribution is given by

$$(\xi^x_{\text{sp},j})^2 \sum_{i=1}^{j-1} \xi^x_{\text{sp},i} \xi^z_{\text{sp},i} (w_j - w_i)$$

with weight $w_j$ close to 1. This shows that unconfounded high frequencies enter the expression in a similar way to non-spatial information.

Therefore, when $\mathbf{x}$ has sufficient non-spatial information or unconfounded high frequencies, then we can generally expect the bias of the non-spatial model to be higher than that of the spatial model, with the difference between the biases larger when there is a lot of confounding at low frequencies. However, the relationship between the two biases is subtle and, when confounding is at high frequencies, the bias in the spatial model could well exceed that of the non-spatial model.

## 1.6 Dependence on the smoothing parameter

We consider here how the expression for the bias given in Corollary 1 depends on the overall level of smoothing controlled by the smoothing parameter $\lambda > 0$. For each $i = 1, \ldots, p$, consider the i'th weight $w_i$ as a function of $\lambda$:

$$w_i(\lambda) = \tfrac{\lambda \alpha_i}{\sigma^{-2} + \lambda \alpha_i}.$$

We see that $\lim_{\lambda \to 0} w_i(\lambda) = 0$ and (unless $\alpha_i = 0$ in which case $w_i(\lambda) \equiv 0$ is constant) $\lim_{\lambda \to \infty} w_i(\lambda) = 1$. We also have that

$$w_i'(\lambda) = \tfrac{\alpha_i \sigma^{-2}}{(\sigma^{-2} + \lambda \alpha_i)^2} \geq 0.$$

Hence, the weights are either constant (and equal to 0) or increasing between 0 and 1.

Let

$$f(\lambda) = \frac{\sum_{i=1}^{p} \xi^x_{\mathrm{sp},i}\xi^z_{\mathrm{sp},i} w_i(\lambda)}{\sum_{i=1}^{n-p} (\xi^x_{\mathrm{ns},i})^2 + \sum_{i=1}^{p} (\xi^x_{\mathrm{sp},i})^2 w_i(\lambda)}$$

denote the bias in the spatial model for a given $\mathbf{x}$ and $\mathbf{z}$ as a function of $\lambda$. We then have that

$$\begin{aligned} f'(\lambda) &= \frac{\left(\sum_{i=1}^{p} \xi^x_{\mathrm{sp},i}\xi^z_{\mathrm{sp},i} w_i'(\lambda)\right)\left(\sum_{i=1}^{n-p} (\xi^x_{\mathrm{ns},i})^2 + \sum_{i=1}^{p} (\xi^x_{\mathrm{sp},i})^2 w_i(\lambda)\right)}{\left(\sum_{i=1}^{n-p} (\xi^x_{\mathrm{ns},i})^2 + \sum_{i=1}^{p} (\xi^x_{\mathrm{sp},i})^2 w_i(\lambda)\right)^2} \\ & \quad - \frac{\left(\sum_{i=1}^{p} (\xi^x_{\mathrm{sp},i})^2 w_i'(\lambda)\right)\left(\sum_{i=1}^{p} \xi^x_{\mathrm{sp},i}\xi^z_{\mathrm{sp},i} w_i(\lambda)\right)}{\left(\sum_{i=1}^{n-p} (\xi^x_{\mathrm{ns},i})^2 + \sum_{i=1}^{p} (\xi^x_{\mathrm{sp},i})^2 w_i(\lambda)\right)^2}. \end{aligned}$$

So the denominator of $f'(\lambda)$ is positive and the numerator is given by

$$\sum_{i,k} \xi^x_{\mathrm{sp},i}\xi^z_{\mathrm{sp},i} w_i'(\lambda)(\xi^x_{\mathrm{ns},k})^2 + \sum_{i,j} \xi^x_{\mathrm{sp},i}\xi^z_{\mathrm{sp},i}(\xi^x_{\mathrm{sp},j})^2 (w_i'(\lambda)w_j(\lambda) - w_j'(\lambda)w_i(\lambda)).$$

To consider the behaviour of the size of the bias, for simplicity assume that all $\xi^x_{\mathrm{sp},i}\xi^z_{\mathrm{sp},i}$ are positive. Then the first term in the numerator of $f'(\lambda)$ is positive. Note that this term is non-zero if and only if $\mathbf{x}$ has non-spatial information. For the second term, we see that

$$\begin{aligned} w_i'(\lambda)w_j(\lambda) - w_j'(\lambda)w_i(\lambda) &= \tfrac{\alpha_i\sigma^{-2}}{(\sigma^{-2}+\lambda\alpha_i)^2}\tfrac{\lambda\alpha_j}{\sigma^{-2}+\lambda\alpha_j} + \tfrac{\alpha_j\sigma^{-2}}{(\sigma^{-2}+\lambda\alpha_j)^2}\tfrac{\lambda\alpha_i}{\sigma^{-2}+\lambda\alpha_i} \\ &= \tfrac{\lambda\alpha_i\alpha_j\sigma^{-2}}{(\sigma^{-2}+\lambda\alpha_i)(\sigma^{-2}+\lambda\alpha_j)}\left(\tfrac{1}{\sigma^{-2}+\lambda\alpha_i} - \tfrac{1}{\sigma^{-2}+\lambda\alpha_j}\right) \\ &= \tfrac{\lambda^2\alpha_i\alpha_j\sigma^{-2}}{(\sigma^{-2}+\lambda\alpha_i)^2(\sigma^{-2}+\lambda\alpha_j)^2}(\alpha_j - \alpha_i). \end{aligned}$$

So the second term of the numerator can be written as

$$\begin{aligned} &\sum_{i,j} \xi^x_{\mathrm{sp},i}\xi^z_{\mathrm{sp},i}(\xi^x_{\mathrm{sp},j})^2 c_{ij}(\lambda)(\alpha_j - \alpha_i) \\ &\quad = \sum_{i<j} \left(\xi^x_{\mathrm{sp},i}\xi^z_{\mathrm{sp},i}(\xi^x_{\mathrm{sp},j})^2 - \xi^x_{\mathrm{sp},j}\xi^z_{\mathrm{sp},j}(\xi^x_{\mathrm{sp},i})^2\right) c_{ij}(\lambda)(\alpha_j - \alpha_i) \end{aligned}$$

where $c_{ij}(\lambda) = c_{ji}(\lambda) = \frac{\lambda^2\alpha_i\alpha_j\sigma^{-2}}{(\sigma^{-2}+\lambda\alpha_i)^2(\sigma^{-2}+\lambda\alpha_j)^2} \geq 0$. Since $\alpha_j - \alpha_i \geq 0$ for $i < j$ this shows that confounding at low frequencies ($\xi^x_{\mathrm{sp},i}\xi^z_{\mathrm{sp},i} \neq 0$) contribute positively to the second term of $f'(\lambda)$ whereas confounding at high frequencies ($\xi^x_{\mathrm{sp},j}\xi^z_{\mathrm{sp},j} \neq 0$) contribute negatively. Conversely, unconfounded high frequencies ($\xi^x_{\mathrm{sp},j} \neq 0$, $\xi^z_{\mathrm{sp},j} = 0$) contribute positively, while unconfounded low frequencies ($\xi^x_{\mathrm{sp},i} \neq 0$, $\xi^z_{\mathrm{sp},i} = 0$) contribute negatively.

Our analysis therefore shows that the function $f(\lambda)$, i.e. the size of the bias in the spatial model as a function of $\lambda$, is quite complicated and the overall shape of the function depends on the confounding scenario. However, if there is a relatively large proportion of non-spatial information or unconfounded high frequency spatial

components in $\mathbf{x}$, then we can expect the behaviour of the first term in the derivative to dominate so that $f(\lambda)$ is (at least broadly) an increasing function, i.e. it is in line with the intuition that more smoothing leads to larger bias.

*Proof of Corollary 3.* From the limiting behaviour of the weights $w_i(\lambda)$, it follows directly that

$$\lim_{\lambda\to\infty} f(\lambda) = \frac{\sum_{\{i|\alpha_i\neq 0\}} \xi^x_{\mathrm{sp},i}\xi^z_{\mathrm{sp},i}}{\sum_{i=1}^{n-p}(\xi^x_{\mathrm{ns},i})^2 + \sum_{\{i|\alpha_i\neq 0\}}(\xi^x_{\mathrm{sp},i})^2}.$$

For the limit as $\lambda \to 0$, we see that $f(\lambda) = \frac{\mathrm{Num}(\lambda)}{\mathrm{Den}(\lambda)}$ where

$$\mathrm{Num}'(\lambda) = \sum_{i=1}^{p} \xi^x_{\mathrm{sp},i}\xi^z_{\mathrm{sp},i} w_i'(\lambda), \quad \mathrm{Den}'(\lambda) = \sum_{i=1}^{p} (\xi^x_{\mathrm{sp},i})^2 w_i'(\lambda).$$

Therefore, using l'Hôspital's rule,

$$\lim_{\lambda\to 0} f(\lambda) = \begin{cases} 0 & \text{if } \boldsymbol{\xi}^x_{\mathrm{ns}} \neq \mathbf{0} \\ \lim_{\lambda\to 0} \frac{\mathrm{Num}'(\lambda)}{\mathrm{Den}'(\lambda)} = \frac{\sum_{i=1}^{p} \xi^x_{\mathrm{sp},i}\xi^z_{\mathrm{sp},i}\alpha_i}{\sum_{i=1}^{p}(\xi^x_{\mathrm{sp},i})^2\alpha_i} & \text{otherwise} \end{cases}.$$

□

Note that in the case where $\mathbf{x}$ has no non-spatial components, the bias doesn't go to 0 as $\lambda \to 0$, however, the limit can still become close to 0 if $\mathbf{x}$ has large unconfounded high frequency components. This is in line with the intuition that unconfounded high frequency components affect the bias in a similar way to non-spatial components.

## 1.7 Variance inflation

The literature on spatial confounding generally focuses on the bias in covariate effect estimates, but some papers (Reich et al., 2006; Zimmerman and Ver Hoef, 2022) also mention "variance inflation" in the spatial model compared to the non-spatial model. This can be explained by the following results.

Firstly, we compute expressions for the variance of the covariate effect estimates in the spatial model (3) and the non-spatial model (4). We see that, as was the case for the bias, the expressions agree except that the spatial model uses the metric defined by $\Sigma^{-1}$ whereas in the non-spatial model, this is replaced by the usual Euclidean metric.

**Proposition A.1.** *Let* $\mathbf{U}$ *be the orthonormal eigenbasis which diagonalises* $\Sigma^{-1}$*, and* $\boldsymbol{\xi}^x = (\boldsymbol{\xi}^{xT}_{\mathrm{ns}}, \boldsymbol{\xi}^{xT}_{\mathrm{sp}})^T$ *the coordinates of* $\mathbf{x}$ *in this basis. The variance of the estimated covariate effect* $\widehat{\beta}$ *in model (3) is given by*

$$\mathrm{Var}(\widehat{\beta}) = \sigma^2 \frac{\langle \mathbf{x}, \mathbf{x}\rangle_{(\Sigma^{-1})^2}}{(\langle \mathbf{x}, \mathbf{x}\rangle_{\Sigma^{-1}})^2} = \sigma^2 \frac{\sum_{i=1}^{n-p}(\xi^x_{\mathrm{ns},i})^2 + \sum_{i=1}^{p}(\xi^x_{\mathrm{sp},i})^2 w_i^2}{\left(\sum_{i=1}^{n-p}(\xi^x_{\mathrm{ns},i})^2 + \sum_{i=1}^{p}(\xi^x_{\mathrm{sp},i})^2 w_i\right)^2},$$

*where* $w_i = \lambda\alpha_i/(\sigma^{-2} + \lambda\alpha_i)$ *for* $i = 1, \ldots, p$.

*Proof.* Since under the data generating model (2)$\text{Var}(\mathbf{y}) = \sigma^2\mathbf{I}$, we have that

$$\begin{aligned} \text{Var}(\widehat{\beta}) &= (\mathbf{x}^T\Sigma^{-1}\mathbf{x})^{-2}\left(\mathbf{x}^T\Sigma^{-1}\right)\text{Var}(\mathbf{y})\left(\mathbf{x}^T\Sigma^{-1}\right)^T \\ &= \sigma^2(\mathbf{x}^T\Sigma^{-1}\mathbf{x})^{-2}\mathbf{x}^T(\Sigma^{-1})^2\mathbf{x} \\ &= \sigma^2\frac{\langle\mathbf{x},\mathbf{x}\rangle_{(\Sigma^{-1})^2}}{(\langle\mathbf{x},\mathbf{x}\rangle_{\Sigma^{-1}})^2}. \end{aligned}$$

As $(\Sigma^{-1})^2$ has eigenvalues $\{\sigma^{-4}, \sigma^{-4}w_1^2, \dots, \sigma^{-4}w_p^2\}$ and is also diagonalised in the eigenbasis $\mathbf{U}$, the result follows (as in the proof of Corollary 1) by writing the above expression in the coordinates $\boldsymbol{\xi}^x$. $\square$

The proof of the following corollary is given in Appendix 1.8 below.

**Corollary A.1.** *Let* $\mathbf{U}$ *be the orthonormal eigenbasis which diagonalises* $\Sigma^{-1}$*, and* $\boldsymbol{\xi}^x = (\boldsymbol{\xi}_{\text{ns}}^{xT}, \boldsymbol{\xi}_{\text{sp}}^{xT})^T$ *the coordinates of* $\mathbf{x}$ *in this basis. The variance of the estimated covariate effect* $\widehat{\beta}_{\text{ns}}$ *in model (4) is given by*

$$\text{Var}(\widehat{\beta}_{\text{ns}}) = \sigma^2\langle\mathbf{x},\mathbf{x}\rangle^{-1} = \frac{\sigma^2}{\sum_{i=1}^{n-p}(\xi_{\text{ns},i}^x)^2 + \sum_{i=1}^{p}(\xi_{\text{sp},i}^x)^2}.$$

Combining Proposition A.1 and Corollary A.1 we get the following results about the variance of the effect estimate in the spatial model.

**Corollary A.2.** *Let* $\mathbf{U}$ *be the orthonormal eigenbasis which diagonalises* $\Sigma^{-1}$*, and* $\boldsymbol{\xi}^x = (\boldsymbol{\xi}_{\text{ns}}^{xT}, \boldsymbol{\xi}_{\text{sp}}^{xT})^T$ *the coordinates of* $\mathbf{x}$ *in this basis. The expressions for the variances* $\text{Var}(\widehat{\beta})$ *and* $\text{Var}(\widehat{\beta}_{\text{ns}})$ *in the spatial and non-spatial model, respectively, satisfy the inequality* $\text{Var}(\widehat{\beta}) \geq \text{Var}(\widehat{\beta}_{\text{ns}})$*. We also have the following limiting behaviour of* $\text{Var}(\widehat{\beta})$*:*

$$\begin{aligned} \lim_{\lambda\to 0}\text{Var}(\widehat{\beta}) &= \frac{\sigma^2}{\sum_{i=1}^{n-p}(\xi_{\text{ns},i}^x)^2}, \\ \lim_{\lambda\to\infty}\text{Var}(\widehat{\beta}) &= \frac{\sigma^2}{\sum_{i=1}^{n-p}(\xi_{\text{ns},i}^x)^2 + \sum_{\{i|\alpha_i\neq 0\}}(\xi_{\text{sp},i}^x)^2}, \end{aligned}$$

*where the limit* $\lambda \to 0$ *assumes that* $\boldsymbol{\xi}_{\text{ns}}^{xT} \neq \mathbf{0}$.

*Proof.* Recall from Appendix 1.6 that each weight $w_i$ has $0 \leq w_i < 1$ and increases as a function of the overall smoothing parameter $\lambda$ with $\lim_{\lambda\to 0} w_i(\lambda) = 0$ and $\lim_{\lambda\to\infty} w_i(\lambda) = 1$. Also, let

$$\begin{aligned} C_{\text{ns}} &= \sum_{i=1}^{n-p}(\xi_{\text{ns},i}^x)^2 \geq 0, \\ c_{\text{sp},i} &= (\xi_{\text{sp},i}^x)^2 \geq 0 \quad \text{for } i = 1, \dots p. \end{aligned}$$

Then Proposition A.1 and Corollary A.1 show that

$$\begin{aligned}
\mathrm{Var}(\widehat{\beta}) &= \sigma^2 \frac{C_{\mathrm{ns}} + \sum_{i=1}^p c_{\mathrm{sp},i} w_i^2}{\left(C_{\mathrm{ns}} + \sum_{i=1}^p c_{\mathrm{sp},i} w_i\right)^2}, \\
\mathrm{Var}(\widehat{\beta}_{\mathrm{ns}}) &= \frac{\sigma^2}{C_{\mathrm{ns}} + \sum_{i=1}^p c_{\mathrm{sp},i}} \\
&= \sigma^2 \frac{C_{\mathrm{ns}} + \sum_{i=1}^p c_{\mathrm{sp},i} w_i^2}{\left(C_{\mathrm{ns}} + \sum_{i=1}^p c_{\mathrm{sp},i}\right)\left(C_{\mathrm{ns}} + \sum_{i=1}^p c_{\mathrm{sp},i} w_i^2\right)}
\end{aligned}$$

So the difference between the two expressions is the denominators:

$$\begin{aligned}
\mathrm{Den}_{\mathrm{sp}} &= \left(C_{\mathrm{ns}} + \sum_{i=1}^p c_{\mathrm{sp},i} w_i\right)^2, \\
\mathrm{Den}_{\mathrm{ns}} &= \left(C_{\mathrm{ns}} + \sum_{i=1}^p c_{\mathrm{sp},i}\right)\left(C_{\mathrm{ns}} + \sum_{i=1}^p c_{\mathrm{sp},i} w_i^2\right).
\end{aligned}$$

Thus, to show that $\mathrm{Var}(\widehat{\beta}_{\mathrm{ns}}) \leq \mathrm{Var}(\widehat{\beta})$, it suffices to show that $\mathrm{Den}_{\mathrm{sp}} \leq \mathrm{Den}_{\mathrm{ns}}$. We have that

$$\begin{aligned}
\mathrm{Den}_{\mathrm{ns}} - \mathrm{Den}_{\mathrm{sp}} &= C_{\mathrm{ns}}^2 + \sum_{i,j=1}^p c_{\mathrm{sp},i} c_{\mathrm{sp},j} w_j^2 + C_{\mathrm{ns}} \sum_{i=i}^p c_{\mathrm{sp},i}(w_i^2 + 1) \\
&\quad - C_{\mathrm{ns}}^2 - \sum_{i,j=1}^p c_{\mathrm{sp},i} w_i c_{\mathrm{sp},j} w_j - 2C_{\mathrm{ns}} \sum_{i=i}^p c_{\mathrm{sp},i} w_i \\
&= \sum_{i,j=1}^p c_{\mathrm{sp},i} c_{\mathrm{sp},j}(w_j^2 - w_i w_j) + C_{\mathrm{ns}} \sum_{i=i}^p c_{\mathrm{sp},i}(w_i - 1)^2 \\
&\geq \sum_{i,j=1}^p c_{\mathrm{sp},i} c_{\mathrm{sp},j}(w_j^2 - w_i w_j) \\
&= \sum_{i<j}^p c_{\mathrm{sp},i} c_{\mathrm{sp},j}(w_j^2 - w_i w_j + w_i^2 - w_j w_i) \\
&= \sum_{i<j}^p c_{\mathrm{sp},i} c_{\mathrm{sp},j}(w_j - w_i)^2 \geq 0.
\end{aligned}$$

Hence $\mathrm{Var}(\widehat{\beta}_{\mathrm{ns}}) \leq \mathrm{Var}(\widehat{\beta})$.

The limits $\lim_{\lambda \to 0} \mathrm{Var}(\widehat{\beta})$ and $\lim_{\lambda \to \infty} \mathrm{Var}(\widehat{\beta})$ follow directly from inserting the limits $\lim_{\lambda \to 0} w_i(\lambda) = 0$ and $\lim_{\lambda \to \infty} w_i(\lambda)$ into the expression for $\mathrm{Var}(\widehat{\beta})$. □

Corollary A.2 appears to prove that the variance in the spatial model is indeed inflated compared to that of the non-spatial model. However, an important note here is that the parameter $\sigma^2$ is usually estimated, and the estimate in the non-spatial model is likely to be somewhat bigger than the estimate in the spatial model (because the spatial

effects approximate the unmeasured spatial variation $\mathbf{z}$ whereas the non-spatial model treats $\mathbf{z}$ as largely unexplained.) Therefore, the estimated variance in the non-spatial model will typically be larger than in the spatial model, and this is in fact what is often seen in practice.

Note that for the same value of $\sigma^2$, the effect of the "variance inflation" tends to be small when either $\lambda$ is large or the proportion of spatial information in $\mathbf{x}$ is small. This is in line with intuition as smoothing is expected to decrease the variance of the spatial model estimates (and large values of $\lambda$ give more smoothing), and less spatial information in $\mathbf{x}$ should lead to less uncertainty around what relates to the covariate as opposed to the spatial effects.

### 1.8 Proof of Corollaries 2 and A.1

*Proof.* The model (4) can be viewed as a spatial model (3) with a single unsmoothed spatial basis vector spanning the intercept, that is, $\mathbf{B}_{\text{sp}} = [b_1]$ where $b_1 = (1, \ldots, 1)^T$ and $w_1 = \alpha_1 = 0$. Inserting this into the expression for $\Sigma^{-1}$ and using the fact that $b_1^T b_1 = n$ then gives that

$$\Sigma^{-1} = \sigma^{-2}(\mathbf{I} - \tfrac{1}{n} b_1 b_1^T), \quad (\Sigma^{-1})^2 = \sigma^{-2}\Sigma^{-1}.$$

Under the assumption that $\mathbf{x}$ is centered we have that $\mathbf{x}^T b_1 = 0$ and, therefore,

$$\langle \mathbf{x}, \mathbf{z} \rangle_{\Sigma^{-1}} = \sigma^{-2}\mathbf{x}^T(\mathbf{I} - \tfrac{1}{n} b_1 b_1^T)\mathbf{z} = \sigma^{-2}\langle \mathbf{x}, \mathbf{z} \rangle.$$

Similarly,

$$\langle \mathbf{x}, \mathbf{x} \rangle_{\Sigma^{-1}} = \sigma^{-2}\langle \mathbf{x}, \mathbf{x} \rangle \quad \text{and} \quad \langle \mathbf{x}, \mathbf{x} \rangle_{(\Sigma^{-1})^2} = \sigma^{-4}\langle \mathbf{x}, \mathbf{x} \rangle.$$

The results then follow from Propositions 1 and A.1. □

## 2 Reparameterisation of spatial effects

In Scenario 3 of the simulation study and when implementing the capped spatial+, we use reparameterisation of the TPRS spatial effect. In this section, we explain how this reparametrisation is obtained. Recall Equation (3) and $\boldsymbol{\beta}_{\text{sp}} \sim N(\mathbf{0}, \lambda^{-1}\mathbf{S}^{-})$. We can use an eigendecomposition to diagonalise $\mathbf{S} = \mathbf{U}\boldsymbol{\Lambda}\mathbf{U}^T$ where $\boldsymbol{\Lambda}$ is a diagonal matrix of the eigenvalues $\alpha_1, \ldots, \alpha_p$ and $\mathbf{U}$ contains the associated eigenvectors. In order to consider, for example, only the $k$ highest frequencies from the spatial effect, we reparameterise the model such that $\tilde{\mathbf{B}}_{\text{sp}} = \mathbf{B}_{\text{sp}}\tilde{\mathbf{U}}$ and $\tilde{\boldsymbol{\beta}}_{\text{sp}} \sim N(\mathbf{0}, \lambda^{-1}(\tilde{\boldsymbol{\Lambda}})^{-})$, where $\tilde{\mathbf{U}}$ and $\tilde{\boldsymbol{\Lambda}}$ are $p \times (p-k)$ and $(p-k) \times (p-k)$ matrices, respectively, associated with $\mathbf{U}$ and $\boldsymbol{\Lambda}$ after removing the columns associated with the $k$ highest frequencies. In Scenario 3 of the simulation study, this reparametrisation is used to generate $\mathbf{z}_{\text{sp,h}}$ and $\mathbf{z}_{\text{sp,l}}$ and in Section 5.4, this reparameterised spatial effect without the $k$ highest frequencies is used in the capped spatial+ in both the first and second order equations.

In Section 5.4, the same method is used to generate $\mathbf{z}^x_{\text{sp,low}}$, $\mathbf{z}^x_{\text{sp,medium}}$, or $\mathbf{z}^x_{\text{sp,high}}$, where we choose the relevant frequencies and reparameterise the spatial effect as described above.

# 3 Additional simulation results

## 3.1 MSE of fitted values

Figure 7 shows the MSE of fitted values for the several models in Scenarios 1–4 of the simulation study as well as the simulations for capped spatial+. For Scenarios 1–4, as expected, the non-spatial model generally has a worse fit than the spatial model as it is mis-specified.

## 3.2 Scenario 3: Comparison to the non-spatial model

Here, we repeat Scenario 1 but with a larger proportion of unconfounded low frequency components in $\mathbf{x}$ so that the correlation between $\mathbf{x}$ and $\mathbf{z}$ is low overall, but high at high frequencies. Specifically, we consider $\xi^x_{\mathrm{sp,h}} = 1$, $\xi^z_{\mathrm{sp,l}} = 0$, $\xi^x_{\mathrm{sp,l}} \in \{1, 20\}$ and $\xi^z_{\mathrm{sp,h}} \in \{0.2, 0.5, 1\}$ (with $\xi^x_{\mathrm{sp,l}} = 1$ corresponding to Scenario 1). For both models, the coefficient $\xi^x_{\mathrm{sp,l}}$ only contributes to the denominator of the bias. In the spatial model, this contribution is multiplied by relatively small weights $w_i$, whereas in the non-spatial model all weights are 1. Therefore, increasing $\xi^x_{\mathrm{sp,l}}$ keeping everything else fixed should reduce the bias in both models, but with a much larger effect on the non-spatial bias. The results in Figure 6 (left) confirm this, and we see that bias in the spatial model now exceeds the non-spatial bias.

# 4 Simulation results using Gaussian Processes in the DGP

In this section we extend the simulation results of Section 4. As an alternative to using the thin plate regression splines to generate low and high frequency spatial fields $\mathbf{z}_{\mathrm{sp,l}}$ and $\mathbf{z}_{\mathrm{sp,h}}$, here we use Gaussian processes. The analysing spatial model still uses thin plate regression splines, thus we are in a mis-specified model setting. Compared to Section 4,mis-specification bias may occur in addition to the confounding bias. However, generally, conclusions in each scenario follow quite closely to those in Section 4.

In order to generate the data, we start by considering a mean-zero Gaussian process $\boldsymbol{\gamma}$ with exponential covariance structure following $C(h) = \exp(-h/\kappa)$ such data $h = \|\mathbf{s} - \mathbf{s}'\|$ for $\mathbf{s}, \mathbf{s}' \in [0, 1] \times [0, 1]$, which is assumed for the sake of simplicity to have variance of 1. We set $\kappa = 0.3$ corresponding to a spatial range of approximately 0.3. Let $\boldsymbol{\Sigma}_{\mathrm{sp}}$ be the positive-definite spatial covariance matrix of $\boldsymbol{\gamma}$ and consider its eigendecomposition $\boldsymbol{\Sigma}_{\mathrm{sp}} = \mathbf{V}_{\mathrm{sp}}\boldsymbol{\Lambda}\mathbf{V}_{\mathrm{sp}}^T$ where $\mathbf{V}_{\mathrm{sp}}$ is an orthogonal matrix of eigenvectors of $\boldsymbol{\Sigma}_{\mathrm{sp}}$ and $\boldsymbol{\Lambda}$ is a diagonal matrix that contains the corresponding eigenvalues in descending order. We take the first 10 largest eigenvalues of $\boldsymbol{\Sigma}_{\mathrm{sp}}$ and define the $\boldsymbol{\Sigma}_{\mathrm{sp,l}} = \mathbf{V}_{\mathrm{sp,l}}\boldsymbol{\Lambda}_l{\mathbf{V}_{\mathrm{sp,l}}}^T$ where $\mathbf{V}_{\mathrm{sp,l}}$ and $\boldsymbol{\Lambda}_l$ are the submatrices of $\mathbf{V}_{\mathrm{sp}}$ and $\boldsymbol{\Lambda}$, respectively, associated with the 10 largest eigenvalues. Let the square root of $\boldsymbol{\Sigma}_{\mathrm{sp,l}}$ be $\mathbf{L}^{1/2}_{\mathrm{sp,l}} = \mathbf{V}_{\mathrm{sp,l}}\boldsymbol{\Lambda}_l^{1/2}{\mathbf{V}_{\mathrm{sp,l}}}^T$. Then, $\mathbf{z}_{\mathrm{sp,l}} = \mathbf{L}_{\mathrm{sp,l}}\boldsymbol{\zeta}_l$ where $\boldsymbol{\zeta}_l$ follows a standard normal distribution. We take the remaining $n - 10$ eigenvalues of $\boldsymbol{\Sigma}_{\mathrm{sp}}$ and define $\mathbf{L}_{\mathrm{sp,h}} = \mathbf{V}_{\mathrm{sp,h}}\boldsymbol{\Lambda}_h^{1/2}{\mathbf{V}_{\mathrm{sp,h}}}^T$ such that $\mathbf{z}_{\mathrm{sp,h}} = \mathbf{L}_{\mathrm{sp,h}}\boldsymbol{\zeta}_h$ where $\boldsymbol{\zeta}_h$ follows a standard

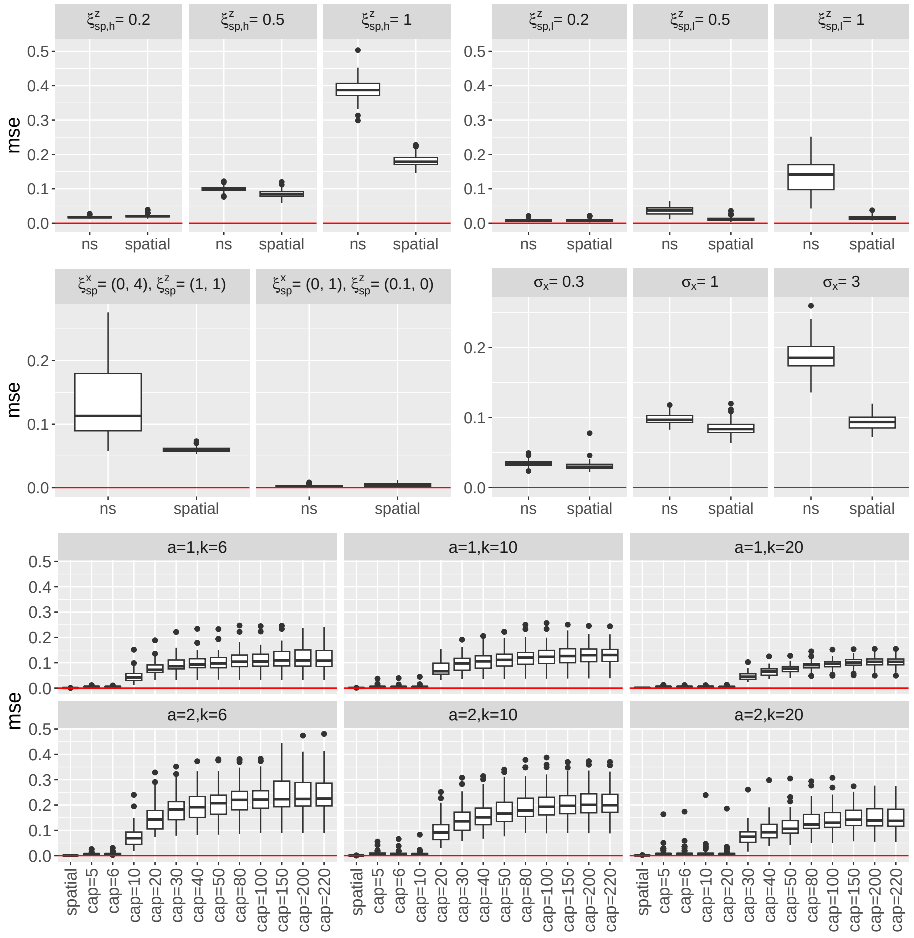

Figure 5: MSE of fitted values in the spatial and non-spatial (ns) models under Scenario 1 (top, left), Scenario 2 (top, right), Scenario 3 (middle, left), Scenario 4 (middle, right). MSE of fitted values in simulations for capped spatial+ (bottom).

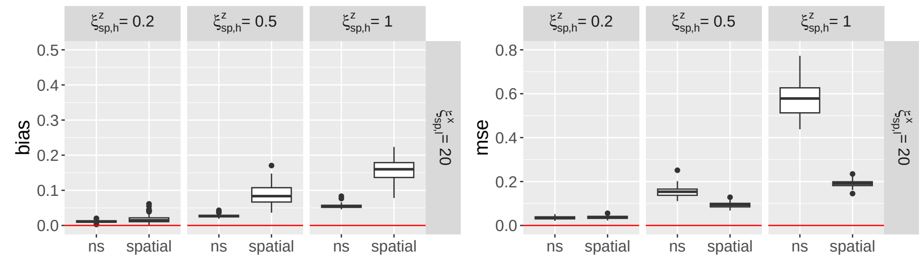


Figure 6: Bias of $\widehat{\beta}$ and $\widehat{\beta}_{\text{ns}}$ (left) and mean squared error of fitted values (right) in the spatial and non-spatial (ns) models under the additional simulations for Scenario 3. The true value of $\beta$ is 0.5.

normal distribution. Note that the spatial covariance matrix of the Gaussian process has full rank $n$ and we use all eigenvalues to generate $\mathbf{z}_{\text{sp,l}}$ and $\mathbf{z}_{\text{sp,h}}$, so the spatial basis vectors span the whole space, i.e the noise term in $\mathbf{x}$ is unconfounded in the sense that it is generated independently from the spatial effect $\mathbf{z}$, but it still is a linear combination of the spatial basis vectors. The spatial analysis model uses thin plate regression splines with 300 basis functions.

Some details are skipped in the following sections as they overlap both in terms of expectations and final conclusions to those in Section 4. For a more detailed reflection on the results, we recommend consulting Section 4.

## 4.1 Scenario 1: Confounding at high frequencies

We consider $(\xi^x_{\text{sp,l}}, \xi^x_{\text{sp,h}}) = (1, 1)$, $\xi^z_{\text{sp,l}} = 0$ and $\xi^z_{\text{sp,h}} \in \{0.5, 2, 3\}$. The results in Figure 7 follow similarly to Scenario 1 in 4. As expected, large contributions to bias in the spatial model happen when there is confounding at high frequencies, and the size of the bias increases linearly with $\xi^z_{\text{sp,h}}$ (as everything else is held fixed). The same logic follows for the non-spatial model and, for this particular data generating process, the bias of the non-spatial model is always larger than the one in the spatial model.

## 4.2 Scenario 2: Confounding at low frequencies

As before, we swap high and low frequencies in $\mathbf{z}$, such that there is only confounding at low frequencies. We consider $(\xi^x_{\text{sp,l}}, \xi^x_{\text{sp,h}}) = (1, 1)$, $\xi^z_{\text{sp,h}} = 0$ and $\xi^z_{\text{sp,l}} \in \{0.5, 2, 3\}$. The results in Figure 7 follow similarly to Scenario 2 in Section 4.When confounding only happens at low frequencies, the bias is close to zero in the spatial model and remains close to zero as $\xi^z_{\text{sp,l}}$ increases, even despite potential model misspecification. Thus, the thin plate regression splines generally seem able to capture the behavior of the Gaussian process used in the data generating process. In contrast, the non-spatial model has a positive and linearly increasing bias, similar to Scenario 2 in Section 4, since all terms are weighted by 1, as opposed to the spatial model where lower frequencies have lower weights.

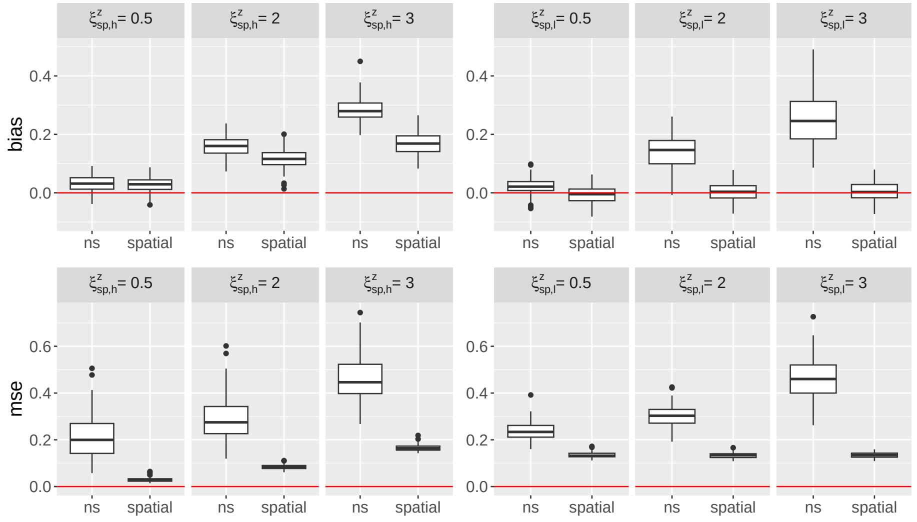

Figure 7: Bias of $\widehat{\beta}$ and $\widehat{\beta}_{\rm ns}$ (top) and mean squared error of fitted values (bottom) in the spatial and non-spatial (ns) models under Scenarios 1 (left) and 2 (right). The true value of $\beta$ is 0.5.

## 4.3 Scenario 3: Comparison to a non-spatial model

We consider $\xi^x_{\rm sp,h} = 1$, $\xi^z_{\rm sp,l} = 0$, $\xi^x_{\rm sp,l} \in \{5, 10\}$ and $\xi^z_{\rm sp,h} \in \{0.5, 2, 3\}$. The results in Figure 8 follow similarly to Scenario 3 in Section 4; by increasing $\xi^x_{\rm sp,l}$ we can reach data generating processes where the non-spatial model has smaller bias than the spatial model, because the correlation between $\mathbf{x}$ and $\mathbf{z}$ is overall low (and thus non-spatial bias is low), but it is strong at high frequencies (inducing high spatial bias).

## 4.4 Scenario 4: Dependence on non-spatial information

We consider $\sigma_x \in \{0.3, 1, 2, 3\}$. Other parameters remain constant at $(\xi^x_{\rm sp,l}, \xi^x_{\rm sp,h}) = (1, 1)$, $(\xi^z_{\rm sp,l}, \xi^z_{\rm sp,h}) = (0, 2)$. The results in Figure 9 follow similarly to Scenario 4 in Section 4 and the bias decreases for both the non-spatial and spatial model when $\sigma_x$ is increased. Once again, the bias is larger in the non-spatial model than in the spatial, except when $\sigma_x = 0.3$.

## 4.5 Scenario 5: Dependence on the smoothing parameter

We consider $(\xi^x_{\rm sp,l}, \xi^x_{\rm sp,h}) = (0, 1)$, $(\xi^z_{\rm sp,l}, \xi^z_{\rm sp,h}) = (1, 1)$, $\sigma_x = \sigma = 1$, and fix $\lambda$ to different values. We let $\sigma_x \in \{0.3, 1, 2\}$. The results are based on 20 replicates.

As can be observed in Figure 10, the higher the $\sigma_x$ the lower the bias. For $\sigma_x = 0.3$, the spatial bias is mostly above the non-spatial bias and slowly converges to the non-spatial bias. Eventually, for $\sigma_x = 2$, the spatial bias is always below the non-spatial bias, until it reaches it for large $\lambda$. Compared to Scenario 5 in Section 4, a bias close

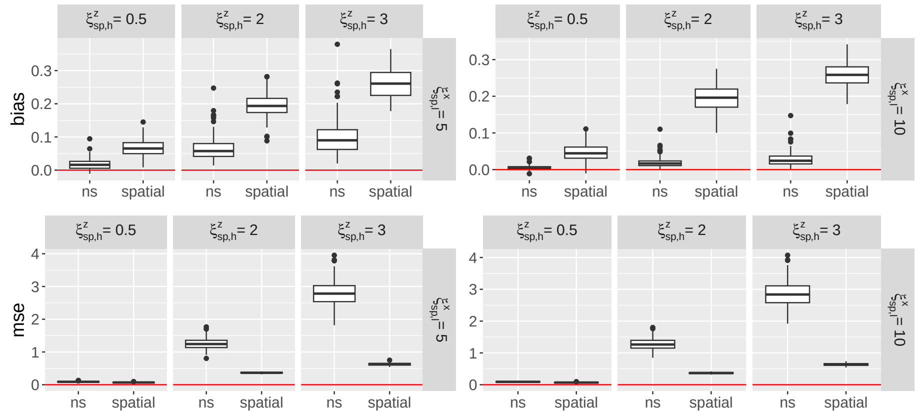


Figure 8: Bias of $\widehat{\beta}$ and $\widehat{\beta}_{\text{ns}}$ (top) and mean squared error of fitted values (bottom) in the spatial and non-spatial (ns) models under Scenario 3. The true value of $\beta$ is 0.5.

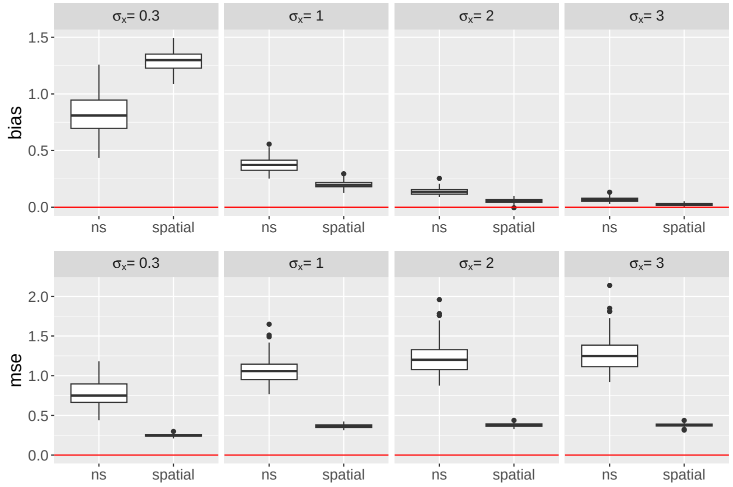


Figure 9: Bias of $\widehat{\beta}$ and $\widehat{\beta}_{\text{ns}}$ (top) and mean squared error of fitted values (bottom) in the spatial and non-spatial (ns) models under Scenario 4. The true value of $\beta$ is 0.5.

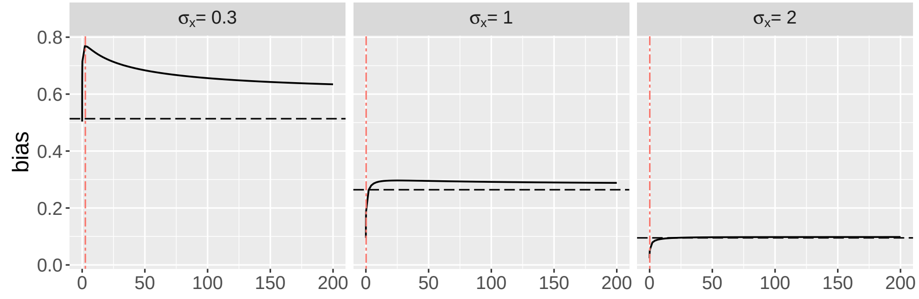


Figure 10: Bias of $\widehat{\beta}$ (solid black) and $\widehat{\beta}_{\mathrm{ns}}$ (dashed black) for increasing $\lambda$ and different $\sigma_x$. The true value of $\beta$ is 0.5. The magenta dashed line shows the median $\hat{\lambda}$ estimated by generalized cross-validation. The bias associated with each $\hat{\lambda}$ is 0.7232, 0.1872, 0.0340, from left to right.

to 0 is never reached for $\sigma_x = 0.3$, most likely due to the presence of additional misspecification bias when using a Gaussian process as the data generating process. The generalized cross-validation estimate $\hat{\lambda}$ always stays on the steep part of the spatial bias curve, indicating that small changes in $\hat{\lambda}$ can lead to large changes in the spatial bias. The $\hat{\lambda}$ for the highest two $\sigma_x$ leads to a spatial bias lower than the non-spatial bias.

# References

Guan, Y., Page, G. L., Reich, B. J., Ventrucci, M., and Yang, S. (2023). Spectral adjustment for spatial confounding. *Biometrika*, 110(3):699—-719.

Keller, J. P. and Szpiro, A. A. (2020). Selecting a scale for spatial confounding adjustment. *Journal of the Royal Statistical Society Series A: Statistics in Society*, 183(3):1121–1143.

Paciorek, C. J. (2010). The importance of scale for spatial-confounding bias and precision of spatial regression estimators. *Statistical Science*, 25(1):107–125.

Page, G. L., Liu, Y., He, Z., and Sun, D. (2017). Estimation and prediction in the presence of spatial confounding for spatial linear models. *Scandinavian Journal of Statistics*, 44(3):780–797.

Reich, B. J., Hodges, J. S., and Zadnik, V. (2006). Effects of residual smoothing on the posterior of the fixed effects in disease-mapping models. *Biometrics*, 62(4):1197–1206.

Zimmerman, D. L. and Ver Hoef, J. M. (2022). On deconfounding spatial confounding in linear models. *The American Statistician*, 76(2):159–167.
